# Supplementary material for: Interacting Stark localization dynamics in a three-dimensional lattice Bose gas
Source: arXiv:2211.12336 ancillary file (2022-11-22)
Supplement: Supplementary file 1 [file Relaxation_of_a_thermal_gas_SM.pdf]

# Supplementary Material: Interacting Stark localization dynamics in a three-dimensional lattice Bose gas

Laura Wadleigh, Nicholas Kowalski, and Brian DeMarco

*Department of Physics, University of Illinois*

*Urbana-Champaign, Urbana, Illinois 61801, USA*

(Dated: November 22, 2022)

## I. INITIAL DENSITY DISTRIBUTION

The frequencies of the trap before turning on the lattice were measured by inducing small oscillations. We determined that one principal axis is oriented vertically with frequency $(73.6 \pm 0.3)$ Hz and the other two are in the horizontal plane with approximately equal frequencies $(48.0 \pm 0.6)$ Hz and $(46.0 \pm 0.8)$ Hz. The additional confinement from the lattice beams is included in modeling the density profile. Given systematic uncertainty, we estimate that the lattice beam waist is $120^{+30}_{-10}$ µm based on the consistency between the lattice beam power, lattice potential depth, and measurements of the forces induced by the envelope of the lattice beams.

The temperature of the initial state $(210 \pm 40)$ nK after turning on the lattice was determined by fitting an in-situ image of the gas to a gaussian function. The central region of the gas where the density is excluded by the barrier potential is masked for this fit, so that the temperature is determined by the tails of the density distribution. The temperature measured using this method was checked by entropy matching [30]. Based on an expansion velocity measurement of the temperature $(115 \pm 10)$ nK before turning on the lattice, the entropy-matched temperature in the lattice is predicted to be $(210 \pm 35)$ nK.

The parameters for the barrier potential were determined by fitting an in-situ image of the gas to a Maxwell-Boltzmann distribution. For this procedure, the overall potential $V$ was modeled as a combination of an attractive harmonic potential and a repulsive potential arising from a focused gaussian laser beam. A measurement of the optical power was used to constrain the magnitude of the barrier potential, leaving just the waist as a free parameter in the fit.

The density distribution of the initial state was modeled via an atomic-limit calculation. The potential energy, including the harmonic confining potential, the barrier potential, and the additional confinement from the $4\,\mathrm{E_R}$ lattice beams, was determined for each lattice site. The number of atoms at each site was determined using the potential energy, interaction energy, and measured temperature for a basis of 0–3 particles and a Maxwell-Boltzmann distribution. An overall chemical potential was varied to match the total atom number. We find that 10% of the atoms are on doubly occupied sites for the initial state. The impact of interactions on the density distribution is small—the RMS size of the gas associated with the tails of the density distribution changes by only 2% for $U = 0$.

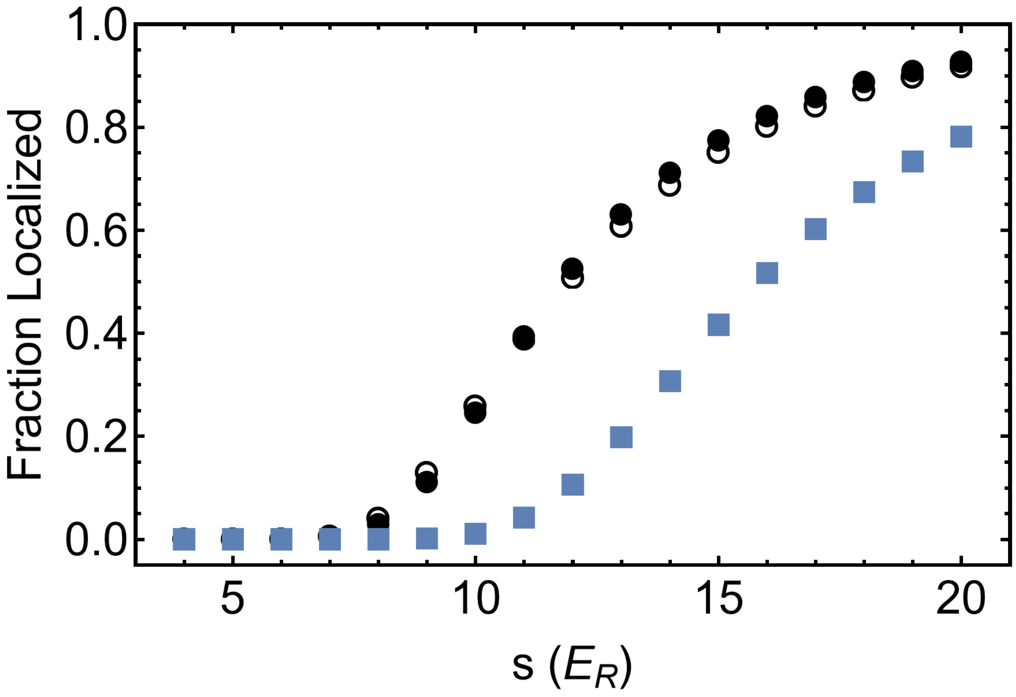


FIG. S1. A lower bound on localization. The blue squares show the fraction of atoms localized to a single lattice site in all three directions. The black circles show the fraction of particles localized along at least one lattice direction. The open and closed circles represent different lattice directions. The slight differences between lattice directions arise because the lattice axes are not aligned to the principal axes of the trap.

## II. LOCALIZATION ESTIMATE

The lower bound on localization was determined by summing the number of atoms on sites where the overall trapping potential gradient is greater than $4t/d$ for the initial state. We carried out this procedure for each direction of the lattice independently. The results are shown in Fig. S1.

To obtain an upper bound on localization, we used exact diagonalization to find the eigenstates of a one-dimensional, single-particle, tight-binding Hamiltonian with a harmonic potential centered on a 300-site lattice. We characterize an eigenstate as delocalized if it

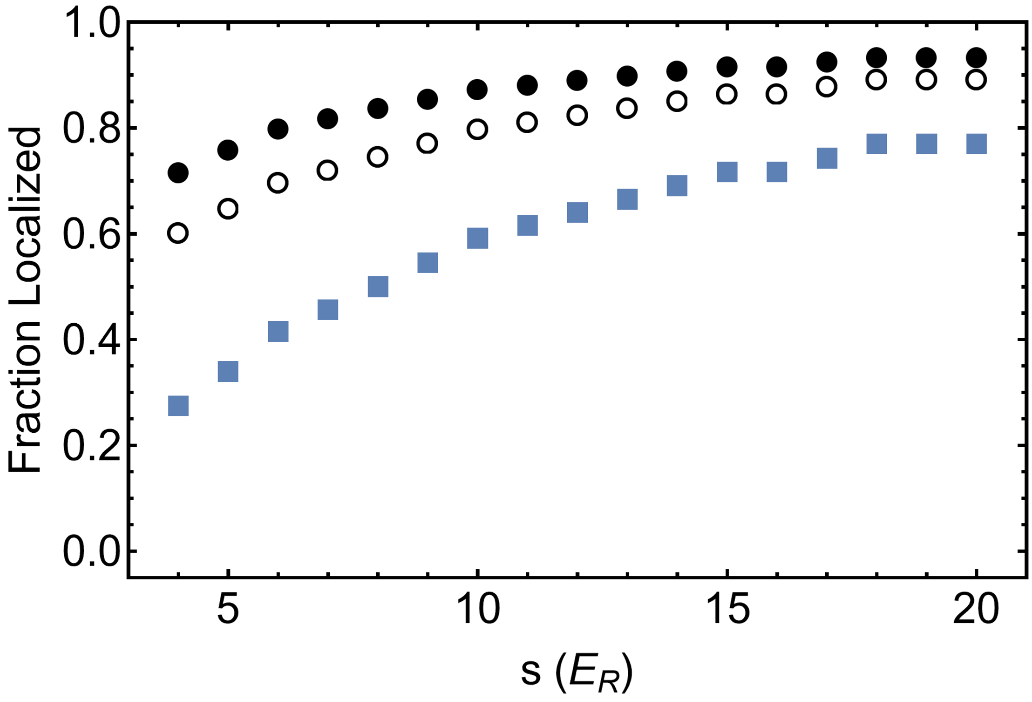


FIG. S2. Upper bound on localization. The blue squares represent the fraction localized in all three directions. The black open circles represent the fraction localized along the direction of the optical barrier propagation and the black filled circles represent the fraction localized along the direction perpendicular to the propagation.

has at least 0.1% probability on the central lattice site. The results are not sensitive to the choice of threshold probability. To determine the fraction of atoms localized in the initial state, we project the Wannier state on each lattice site onto the energy eigenstate basis. We average the localized probability on each lattice site weighted by the number density distribution (Fig. S2).

In order to produce an average across the atomic density distribution, we treat the wavefunctions as separable (i.e., products of wavefunctions that depend on one coordinate only). The fraction of the atomic wavefunction that is localized at each site is determined for each direction independently. The measure of the localization fraction for all three directions is calculated by multiplying together the localization fraction in each direction (for each

lattice site). The averages shown in Fig. S2 are calculated using the three-dimensional number-density distribution as a weight.

For this upper bound calculation of localization, we find that approximtely 70% of the particles are localized in at least one direction, even for the lowest lattice depths. The localization fraction increases with lattice depth to a plateau near 95% for the most localized direction (Fig. S2).

## III. MARDIA'S $B$ STATISTIC

The calculation of Mardia's $B$ statistic is sensitive to imaging noise. To reduce these effects, a defringing technique was applied to the images [31]. Furthermore, a mask was used to calculate $B$ for only the region of the image with sufficient signal-to-noise ratio. The mask was determined by fitting the tails of the distribution to a gaussian in an elliptical coordinate system with the angle of the axes as a free parameter. The mask was applied at three times the RMS radii from this fit. This procedure provides a balance that eliminates nearly all background noise while only introducing a small systematic shift. The shift in $B$ for a gaussian distribution based on this procedure is $-0.07$, which was determined by applying this procedure to generated images of perfect gaussians. To check the validity of Mardia's $B$ statistic as a measure of equilibrium, we measured $B$ for several equilibrium gases with no barrier potential present. We find that $B$ ranges from $-0.10$ to $-0.05$, which is consistent with the value for a masked, ideal gaussian distribution.

## IV. NON-INTERACTING DYNAMICS

In a harmonically trapped system with a free-particle distribution, the phase-space distribution describing the position and momentum of non-interacting particles rotates at the trap frequency. These dynamics will not lead to relaxation. The dynamics in a system with a lattice dispersion is more complex, and it is possible that dephasing of trajectories could mimic a gaussian density distribution at long times.

To rule out this scenario, we simulate semi-classical dynamics for non-interacting particles with a lattice dispersion confined in a parabolic trap. We work in two dimensions and use a symmetric trap with a frequency corresponding to the geometric mean trap frequency in

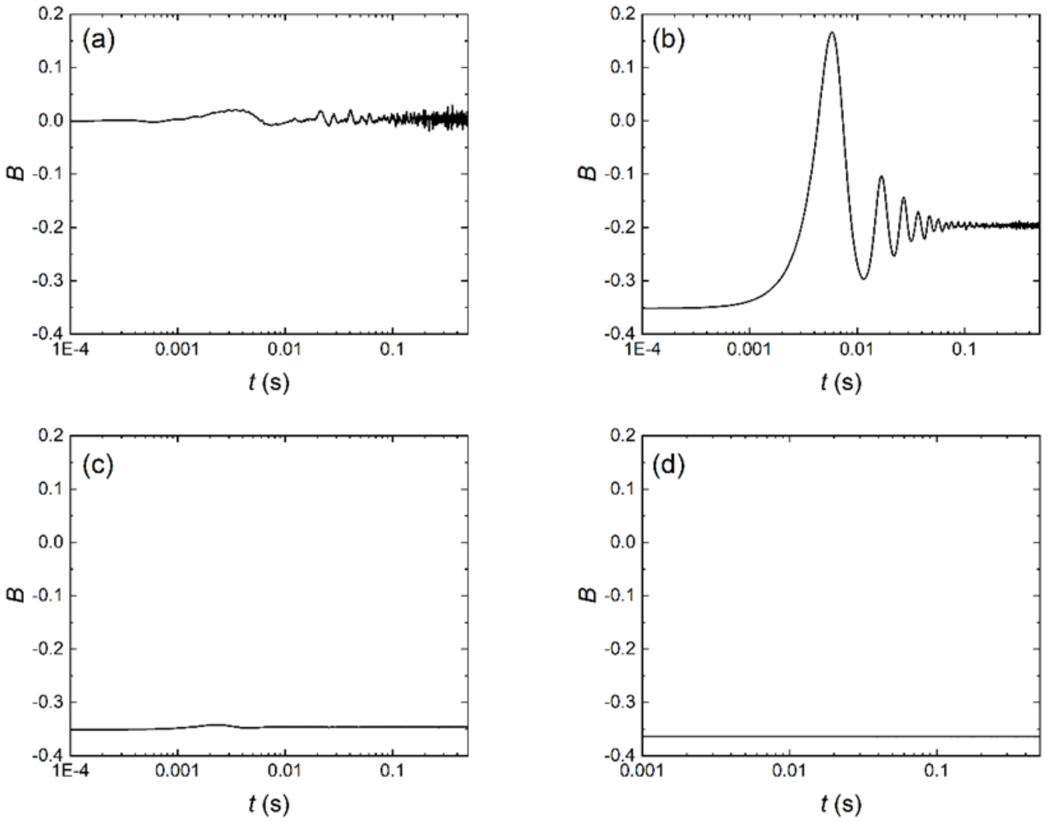


FIG. S3. Simulation of semi-classical dynamics. Two scenarios are simulated at much lower temperature (20 nK) compared with the experiment for $s = 4\,\mathrm{E_R}$: (a) an initial condition at equilibrium and without the barrier and (b) an out-of-equilibrium distribution produced using the barrier potential. Simulations for 200 nK at $s = 4\,\mathrm{E_R}$ and $s = 20\,\mathrm{E_R}$ are shown in panels (c) and (d).

the experiment. In the simulation, the lattice axes are rotated from the trap axes by 47 degrees; we find that the results are not sensitive to this angle. The initial conditions for 10 000 particles are chosen randomly from a Maxwell-Boltzmann distribution that includes the barrier potential.

Euler's method is used to simulate the motion of each particle according to Newton's equation for time $t$. Mardia's $B$ statistic is determined for a column-integrated density distribution. The results of this simulation are shown in Fig. S3. To probe dynamics in a system with relatively few localized states, the dynamics are simulated at $s = 4\ E_R$ for

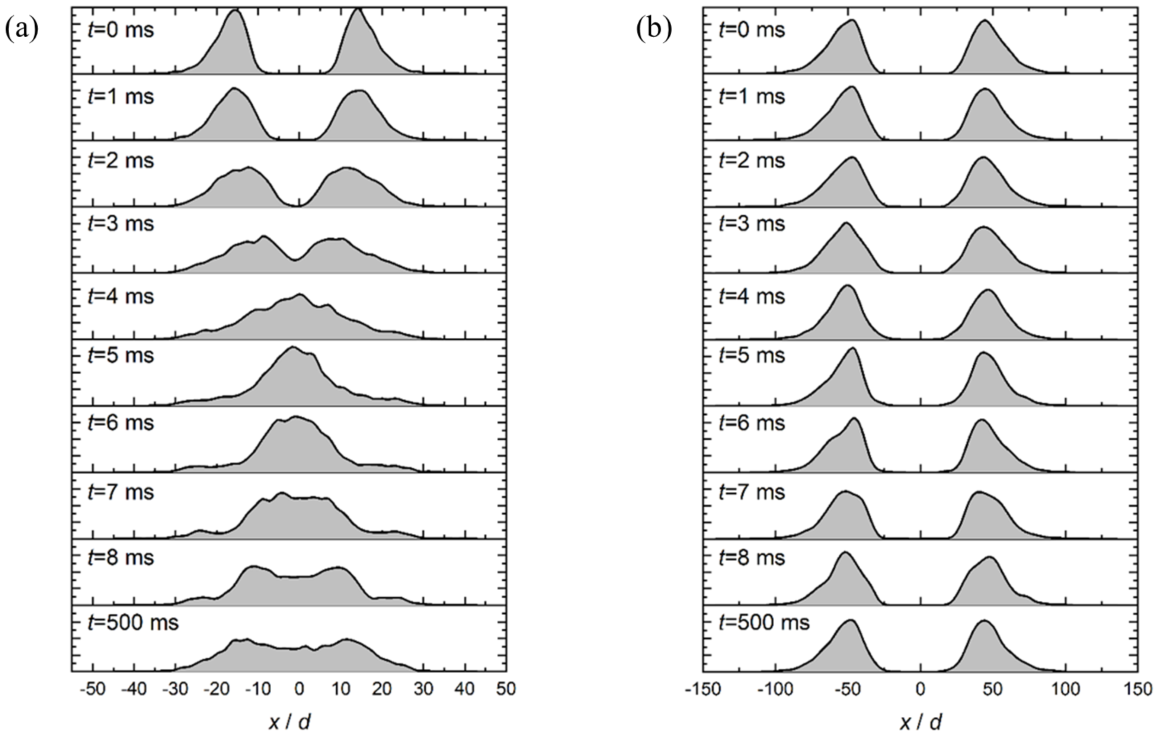


FIG. S4. Simulation of the time-dependent column-integrated density profile for a 20 nK (a) and 200 nK (b) gas.

20 nK, which is much lower temperature compared with the experiment, $(210 \pm 40)$ nK. For the equilibrium case, the dynamics preserve the initial distribution (Fig. S3(a)). In contrast, initial dynamics for the out-of-equilibrium case settle into stationary, but not equilibrium, behavior after approximately 0.1 s (Fig. S3(b)).

The short-time dynamics are suppressed in the higher temperature regime explored by the experiment. Simulations for 200 nK at $s = 4\,\mathrm{E_R}$ and $s = 20\,\mathrm{E_R}$ are shown in panels (c) and (d) of Fig. S3. At these temperatures, a quasi-static distribution is achieved at short times. Furthermore, dynamics present at low lattice depth disappear for stronger lattices.

Snapshots of the column-integrated density profile for 20 nK (Fig. S4(a)) and 200 nK (Fig. S4(b)) at $s = 4\,\mathrm{E_R}$ provide more information about the difference between the low and high-temperature cases. At low temperatures, many particles are free to move, and the short-time dynamics are similar to the free-particle case. Eventually, the lattice dispersion leads

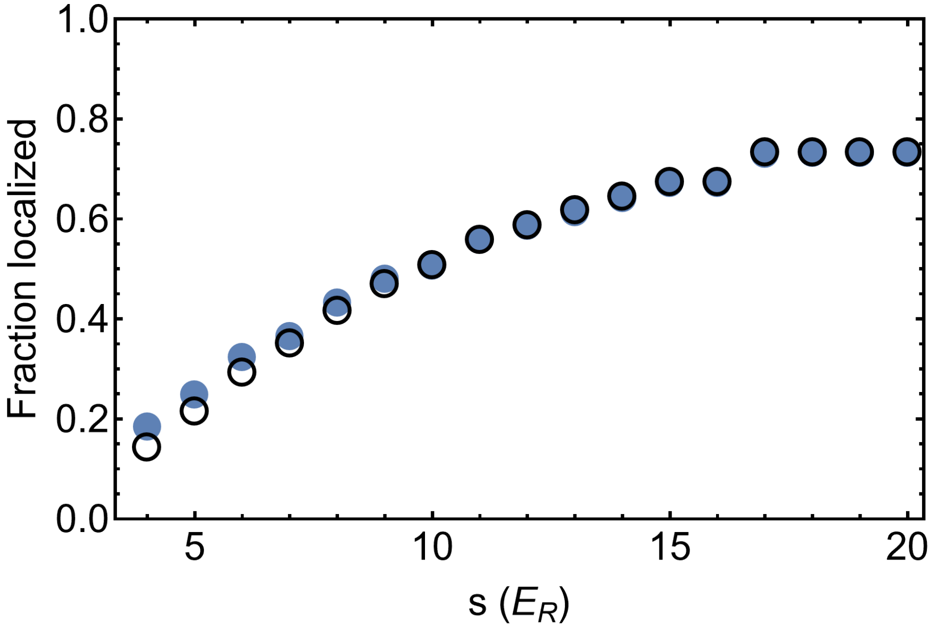


FIG. S5. Fraction of atoms localized for interacting (open, black) and non-interacting (closed, blue) atoms for the equilibrium distribution.

to dephasing of particle trajectories and a non-equilibrium stationary density distribution emerges. For higher temperatures or stronger lattices, most of the particles are Stark-localized, motion is not possible, and the initial density distribution is preserved to long times.

## V. INTERACTION EFFECTS

We carried out an exact calculation to probe the impact of interactions on localization. We created a set of basis states consisting of all possible configurations of two particles populating a one-dimensional, 60-site lattice centered on a parabolic potential. The Bose-Hubbard Hamiltonian was diagonalized using this set of basis states. We defined eigenstates with less than 0.001% probability on the central lattice site as localized. We determined a localization fraction averaged over the equilibrium distribution by taking the thermal average of the eigenstates at the measured long-time temperature (which depends on $s$). The results

of this calculation vary by less than 10% for a range of 0.0002% to 0.005% in the probability threshold for localization.

We find that interactions modify the localized fraction at low lattice depths but do not affect localization at high lattice depths (Fig. S5). The small influence of interactions may, in part, be due to the relatively small presence of doubly occupied sites. For the final state at $4\,\mathrm{E_R}$ ($20\,\mathrm{E_R}$), we estimate that 5% (2%) of atoms are are located on a doubly occupied site.

## VI. TEMPERATURE OF THE FINAL STATE

Since removing the potential barrier is diabatic, we expect that the final-state temperature will be larger compared with the initial state. Furthermore, increasing the lattice potential adds potential energy from added parabolic confinement, and the lattice light heats the atoms.

To check that the final state is consistent with these effects, we calculated the equilibrium temperature by matching the total energy per particle. We used a three-dimensional atomic limit calculation and Maxwell-Boltzmann statistics for a basis involving 0–3 atoms per site. An overall chemical potential was used to match particle number. We computed the energy per particle for the initial state, added the potential energy from increasing the lattice potential depth, and incorporated heating from lattice-light scattering [28]. We determined the final-state temperature needed to match the resulting energy per particle. For a 10-second hold time, we find an expected temperature of $(390 \pm 40)\,\mathrm{nK}$ for a $4\,\mathrm{E_R}$ lattice and $(1200 \pm 120)\,\mathrm{nK}$ for a $20\,\mathrm{E_R}$ lattice.

We compare the expected temperature to the temperature determined by fitting images obtained at 10 s to a gaussian distribution. At $s = 4\ E_R$, the measured temperature is $(390 \pm 40)\,\mathrm{nK}$, which agrees with our estimate. At $s = 20\ E_R$, the measured temperature of $(700 \pm 180)\,\mathrm{nK}$ below our expectation. This discrepancy may be accommodated by atom loss, which can lead to a cooling process that competes with heating. Since atom loss is driven by lattice-light scattering for our experiment (the vacuum-limited lifetime exceeds 5 minutes), this effect will be stronger at higher lattice potential depths. We measure that approximately 40% of the atoms are lost after 10 s at $s = 8\ E_R$.
